# Supplementary material for: Online Authentication Habits of Indian Users
Source: arXiv:2501.14330 source file (2025-01-24)
Supplement: Supplementary file 1 [file appendix.tex]

\label{appendix}
\begin{markdown}
# Survey Material
## 1. Participant Information Sheet
**Title of the study: Survey on Authentication Schemes: Password Managers and 2FA**

**What is the purpose of the study?**  
We aim to understand digital literacy and online security threat awareness in India. How the digital literacy and awareness of online risks changes with user demographics. How aware is the user about the different mitigation techniques and also about various services available to the user for implementing the same. Lastly, after being made aware of these services does it actually make the user feel safe and easy to use?

**What is my role as a participant?**  
As a participant, you will have to answer or fill in the survey with **honesty and integrity**. There will be tutorial videos which you have to follow and implement the steps yourself and fill in your opinion about the ease of use of these services. The questions are about your choice of passwords, and how you store your passwords. How safe and dangerous do you think the digital space in India is and what steps have you taken for its mitigation. The survey is **about 15-20 minutes long** thus your patience will be of paramount importance.

**What are the risks and discomforts associated with the study?**  
There are no risks associated as the survey merely asks about your practices and thoughts about your method of authentications and your preferences on various service providers. On the contrary this survey gives you an opportunity to learn about the potential risks that exist in the digital space today and provides you with tools which easily implement the mitigation techniques.

**Do I have the right to withdraw?**  
Yes, you can withdraw anytime- before, during or even after the survey. Please feel
free to ask any of the co-investigators to pause the survey or end it at any time. You can also choose to skip a particular question if you do not feel comfortable answering it.

**What is the confidentiality policy?**  
All questions asked in the survey do not require specific personal information. All questions are generic which ties the participant to a demographic based on the area of permanent residence and occupation. Everything that you have answered will solely be used for research purposes. **It is to be noted that your bank account and/or UPI details are collected in order to facilitate your reimbursement.**

Consent to participate in this study is voluntary. Any data collected from this study will
only be used for the purpose of academic research.
The names of the Co-Investigators, Principal Investigator and Member Secretary have been hidden due to anonymity.

## 2. Important Information Regarding Our Online Behavior Survey
We appreciate your willingness to participate in our online behavior survey, designed to better understand general online trends and habits. We want to assure you that your privacy and data security are of utmost importance to us.

Before you proceed with the survey, we would like to provide you with some important information:

1. **Anonymity and Privacy Protection**: Rest assured, we are not collecting any specific personal information from you during this survey. Your responses will be treated with strict confidentiality, and we have implemented robust data protection measures to safeguard your privacy.
1. **Generic Information**: All the questions in this survey are designed to gather generic information about online behavior and trends. We are interested in understanding the collective habits and preferences of internet users as a whole, rather than focusing on individual data.
1. **Voluntary Participation**: Your participation in this survey is entirely voluntary. You have the freedom to skip any question you are uncomfortable with, and your decision to participate or not will not have any impact on your relationship with our organization.
1. **Data Usage**: The data collected from this survey will be used solely for research and analytical purposes. It will help us gain valuable insights into online behavior patterns, which will, in turn, contribute to improving online experiences for everyone.
1. **Data Retention**: We will retain the survey data for a limited period necessary for analysis and will then securely dispose of it.

Thank you for your cooperation and trust in our research efforts. Your input is invaluable to us, and it will be used responsibly to enhance our understanding of online behavior. 

Details of the contact person have been hidden due to anonymity.

Your contribution to this research is highly appreciated, and we look forward to your participation.

## 3. Demographic Information
1. Your age group:  
	- [ ] Under 18
	- [ ] 18-25
	- [ ] 26-35
	- [ ] 36-45
	- [ ] 46-55
	- [ ] 56 and above
2. Gender:
	- [ ] Female
	- [ ] Male
	- [ ] Non-binary
	- [ ] Prefer not to say
3. Occupation: _________________________________________
4. Highest Educational Qualification
	- [ ] High School or Below
	- [ ] Bachelor's Degree
	- [ ] Master's Degree
	- [ ] Doctorate Degree
	- [ ] Prefer not to say
	- [ ] Other: _______________________________
5. State Of Permanent Residence: _________________________________________
6. Type of Region of Residence
	- [ ] Rural
	- [ ] Semi-urban
	- [ ] Urban
	- [ ] Prefer not to say
	
## 4. Digital Footprint
7. How many different online accounts do you have:  
Mark only one oval.
	- [ ] 1-5
	- [ ] 6-10
	- [ ] 11-20
	- [ ] 20+
	- [ ] Prefer not to say
8. Primarily, on what type of device do you use websites?  
Check all that apply.
	- [ ] Mobile / Smartphone
	- [ ] Tablet
	- [ ] Personal Computer / Laptop
	- [ ] Gaming Consoles
	- [ ] SmartTV
	- [ ] Prefer not to say
	- [ ] Other: _______________________________
9. What percentage of online accounts have been created by others for you?  
Mark only one oval.
	- [ ] 0%
	- [ ] Less than 50%
	- [ ] More than 50%
	- [ ] 100%
	- [ ] Prefer not to say
10. How regularly do you log in using passwords to any of your online accounts?  
Mark only one oval.
	- [ ] Daily
	- [ ] Weekly
	- [ ] Monthly
	- [ ] Yearly
	- [ ] Never
	- [ ] Prefer not to say
	- [ ] Other: _______________________________
11. On a daily basis how many different passwords do you use for login?  
Mark only one oval.
	- [ ] 1-5
	- [ ] 6-10
	- [ ] More than 10
	- [ ] Prefer not to say
	- [ ] Other: _______________________________
12. On a monthly basis how many different passwords do you use to login?  
Mark only one oval.
	- [ ] 1-5
	- [ ] 6-10
	- [ ] 11-20
	- [ ] More than 20
	- [ ] Prefer not to say
	- [ ] Other: _______________________________
## 5. More on your digital footprint
13. How many of your online accounts share the same password?  
Mark only one oval.
	- [ ] 0%
	- [ ] Between 0% and 25%
	- [ ] Between 25% and 50%
	- [ ] Between 50% and 75%
	- [ ] Between 75% and 100%
	- [ ] Prefer not to say
14. Have you ever forgotten a password for any of your online accounts?  
Mark only one oval.
	- [ ] Yes
	- [ ] No
	- [ ] Prefer not to say
	- [ ] Maybe
15. Do you write down any of your account’s passwords in any **electronic form**?  
Mark only one oval.
	- [ ] No
	- [ ] Yes, only for some accounts
	- [ ] Yes, for all accounts
	- [ ] Prefer not to say
16. Do you write down any of your account’s passwords in any **physical form**?  
Mark only one oval.
	- [ ] No
	- [ ] Yes, only for some accounts
	- [ ] Yes, for all accounts
	- [ ] Prefer not to say
17. How often do you change your passwords for online accounts?  
Mark only one oval.
	- [ ] Monthly
	- [ ] Quarterly
	- [ ] Yearly
	- [ ] Never
	- [ ] Prefer not to say
	- [ ] Other: _______________________________

## 6. Just a bit more on your digital footprint
18. As per National Cyber Security Center (U.K.), the most common password used is “123456” as found in leaked data from various hacks.  
Select all the types of generic passwords you have ever used in the past:  
	- [ ] Sequential numbers like "123456"
	- [ ] Repeating digits like "0000"
	- [ ] Keyboard patterns like "Qwerty" , “ASDFG”
	- [ ] Simple terms like "Password"
	- [ ] Basic terms with numeric suffixes like "Password123"
	- [ ] Personal names
	- [ ] Phone numbers
	- [ ] Beloved fictional characters
	- [ ] Sports-related terms
	- [ ] Birthdays
	- [ ] Common phrases like "LetMeIn"
	- [ ] Song lyrics or quotes like "ImagineAllThePeople"
	- [ ] Pet names or pet-related terms
	- [ ] Favorite movie or book titles
	- [ ] Acronyms of memorable phrases
	- [ ] Abbreviations of personal information
	- [ ] Seasonal terms like "Summer2023"
	- [ ] Random dictionary words
	- [ ] None
	- [ ] Prefer not to say
19. Which password length do you generally prefer?  
Mark only one oval.
	- [ ] Less than 8 characters
	- [ ] 8 to 15 characters
	- [ ] More than 15 characters
	- [ ] Prefer not to say
20. Many websites require certain password policies when you create a password. Do you have a fixed set of rules or a template that you use to generate passwords?  
Mark only one oval.
	- [ ] Yes
	- [ ] No
	- [ ] Prefer not to say

## 7. Two Factor Authentication
This section will consist of questions on Two-factor Authentication (2FA)

21. Are you familiar with Two-Factor Authentication (2FA)?  
Mark only one oval.
	- [ ] Yes
	- [ ] No
	- [ ] Prefer not to say
	- [ ] Maybe
22. Have you ever used Two-Factor Authentication (2FA) for your online accounts?  
(Like for logging into your amazon account, first you've to put your amazon account password, followed by an OTP sent to your phone)  
Mark only one oval.
	- [ ] Yes
	- [ ] No
	- [ ] Prefer not to say
	- [ ] Maybe
23. Which types of authentication schemes have you used or came across for 2FA?  
Check all that apply
	- [ ] PIN
	- [ ] Authentication apps (like Google Authenticator or Duo)
	- [ ] OTP
	- [ ] Hardware Key (maybe a small USB dongle that you plug into your device, or tap via NFC)
	- [ ] Biometrics
	- [ ] Prefer not to say
	- [ ] Other: _______________________________
24. Do you feel that using 2FA enhances online security?  
Mark only one oval.
	- [ ] Strongly agree
	- [ ] Agree
	- [ ] Neutral
	- [ ] Disagree
	- [ ] Strongly disagree
	- [ ] Prefer not to say
25. Have you ever **used** 2FA for **Social Media** Accounts?  
Mark only one oval.
	- [ ] Yes
	- [ ] No
	- [ ] Prefer not to say
	- [ ] Maybe
26. Have you ever **used** 2FA for **Online Banking** Accounts? (mostly banks rely on Password + OTP for login)  
Mark only one oval.
	- [ ] Yes
	- [ ] No
	- [ ] Prefer not to say
	- [ ] Maybe
27. How comfortable do you feel using 2FA on your online accounts?  
Mark only one oval.
	- [ ] Very comfortable
	- [ ] Comfortable
	- [ ] Somewhat uncomfortable
	- [ ] Not very comfortable
	- [ ] Not at all Comfortable
	- [ ] Prefer not to say

## 8. Let's see: What is Two-Factor Authentication (2FA)?
What is 2FA?

28. After this video on 2FA, how confident do you feel about using them?  
Mark only one oval.
	- [ ] Not Confident at all
	- [ ] Not very confident
	- [ ] Somewhat confident
	- [ ] Confident
	- [ ] Very Confident
	- [ ] Prefer not to say
## 9. How to setup 2FA: Google Authenticator App for Gmail:
How to enable 2FA

29. How easy do you find adding 2FA to your online accounts?  
Mark only one oval.
	- [ ] Very Easy
	- [ ] Easy
	- [ ] Somewhat easy
	- [ ] Not very easy
	- [ ] Not at all
	- [ ] Prefer not to say

## 10. Your views on 2FA
30. After the tutorials, Give a preference for each authentication method (0 not at all - 5 very likely)  
Answers must be between 0 and 5.
    - PIN _____________
    - OTP through SMS _____________
    - OTP through Email _____________
    - Hardware Keys _____________
    - Authentication apps (like Google authenticator or Duo) _____________
    - Biometrics (i.e. fingerprint, face, iris) _____________

31. Are you more likely to use Two-Factor Authentication (2FA) for your accounts after seeing these videos?  
Mark only one oval.
	- [ ] Yes, significantly
	- [ ] Yes
	- [ ] Neutral
	- [ ] No
	- [ ] No, not at all
	- [ ] Prefer not to say
32. How likely are you to recommend 2FA to your friends or colleagues after seeing the videos?  
Mark only one oval.
	- [ ] Very likely
	- [ ] Likely
	- [ ] Neither likely nor unlikely
	- [ ] Unlikely
	- [ ] Very unlikely
	- [ ] Prefer not to say
33. What aspects of 2FA do you find most valuable?  
Check all that apply.
	- [ ] Added security layer
	- [ ] Peace of mind
	- [ ] Increased control over account access
	- [ ] Prefer not to say
	- [ ] Other: _______________________________
34. How comfortable are you with creating and managing the accounts using 2FA after the videos/tutorials?  
Mark only one oval.
	- [ ] Very comfortable
	- [ ] Comfortable
	- [ ] Neither comfortable nor uncomfortable
	- [ ] Uncomfortable
	- [ ] Very uncomfortable
	- [ ] Prefer not to say
	
## 11. There are 2FA vendors other than Google!
There are some other 2FA services like Duo (for general applications) and Steam Guard (for Steam, an online videogame store) which link your account to a particular device.

Every time you try to login, you have to enter a code generated by your device. 

Alternatively, you might get a push notification to authenticate yourself.

35. In light of the above information, do you believe such methods are more secure than OTPs?  
Mark only one oval.
	- [ ] Yes
	- [ ] No
	- [ ] Prefer not to say
	- [ ] Maybe
36. In case you misplace the device to which your 2FA is linked, what alternate way of logging into the service feels more appropriate?  
Mark only one oval.
	- [ ] Sending an OTP to registered email
	- [ ] Security questions
	- [ ] Backup Codes
	- [ ] Prefer not to say
	- [ ] Other: _______________________________
37. Would you prefer the 2FA application to support data sync across multiple devices?  
Mark only one oval.
	- [ ] No
	- [ ] Yes
	- [ ] Maybe
	- [ ] Prefer not to say
38. Do you believe you need 2FA (reset link + some other verification) during the password reset process?  
Mark only one oval.
	- [ ] No
	- [ ] Yes
	- [ ] Prefer not to say
	- [ ] Maybe
	
## 12. Password Managers
39. Have you observed pop-ups in your web browser suggesting saving passwords for websites?
(Like in the attached image)   
Mark only one oval.
	- [ ] Yes
	- [ ] No
	- [ ] Prefer not to say
	- [ ] Maybe
40. Have you used password-saving feature suggested by the browsers in the past?
(Like in the attached image)  
Mark only one oval.
	- [ ] Yes
	- [ ] No
	- [ ] Prefer not to say
	- [ ] Maybe
41. Have you ever saved your **Internet Banking** password in the password-saving feature suggested by the browsers in the past?  
Mark only one oval.
	- [ ] Yes
	- [ ] No
	- [ ] Prefer not to say
	- [ ] Maybe
42. Have you ever saved your **Social Media** account passwords in the password-saving feature suggested by the browsers in the past?  
Mark only one oval.
	- [ ] Yes
	- [ ] No
	- [ ] Prefer not to say
	- [ ] Maybe
43. Have you ever saved your **e-commerce** websites (Amazon, Flipkart, etc.) password in the password-saving feature suggested by the browsers in the past?  
Mark only one oval.
	- [ ] Yes
	- [ ] No
	- [ ] Prefer not to say
	- [ ] Maybe
	
## 13. More on Password Managers
44. Have you **observed** your web browser generating random passwords for websites during the sign up process?
(Like in the attached image)  
Mark only one oval.
	- [ ] Yes
	- [ ] No
	- [ ] Prefer not to say
	- [ ] Maybe
45. Have you ever **created** a password using the suggestions provided by the browsers/google auto-fill/apple keychain?  
Mark only one oval.
	- [ ] Yes
	- [ ] No
	- [ ] Prefer not to say
	- [ ] Maybe
46. Have you ever **noticed** your app/browser/password-manager **suggesting your saved passwords** while logging into your online account(s)?
(Like in the attached image)  
Mark only one oval.
	- [ ] Yes
	- [ ] No
	- [ ] Prefer not to say
	- [ ] Maybe
47. Have you ever used any password manager(s)?  
Mark only one oval.
	- [ ] Yes
	- [ ] No Skip to question 51
	- [ ] Maybe
	- [ ] Prefer not to say
48. Currently, do you use any password manager(s)?  
Mark only one oval.
	- [ ] Yes
	- [ ] No Skip to question 51
	- [ ] Maybe
	- [ ] Prefer not to say
49. Which password manager(s) do you currently use?  
Check all that apply
	- [ ] Password Managers built-in the browser
	- [ ] Device default managers like: Google Auto-Fill or Apple Keychain
	- [ ] Dedicated third-party manager(s)
	- [ ] Prefer not to say
	- [ ] Not sure
	- [ ] Other: _______________________________
50. Why do you use a password manager?  
Check all that apply.
	- [ ] Auto-filling passwords is convenient
	- [ ] I want my passwords accessible in one place
	- [ ] I don’t want to remember passwords
	- [ ] I remember my passwords but password manager is a backup
	- [ ] My passwords are too complex to remember
	- [ ] I feel safer using a password manager
	- [ ] Prefer not to say
	- [ ] Other: _______________________________

**If you answered Q.50, skip to section 18 (A quick look at the Password Managers)**

51. What is your reason for not using a password manager?  
Check all that apply.
	- [ ] I remember all my passwords
	- [ ] My passwords are simple enough to remember
	- [ ] I reuse my passwords
	- [ ] I feel password-managers unintuitive/hard to use
	- [ ] I do not trust password managers
	- [ ] I write all my passwords somewhere non-digitally
	- [ ] I used password-managers in the past, not anymore
	- [ ] Prefer not to say
	- [ ] Other: _______________________________
	
## 14. A quick look at the Password Managers
Please scan the code and view the video:  

## 15. Setting up Password Managers
How to setup dedicated third-party password manager:  

52. Using a password manager makes logging into websites easier / convenient.  
Mark only one oval.
	- [ ] Strongly Agree
	- [ ] Agree
	- [ ] Neutral
	- [ ] Disagree
	- [ ] Strongly Disagree
	- [ ] Prefer not to say
53. Using a password manager makes logging into websites safer.  
Mark only one oval.
	- [ ] Strongly Agree
	- [ ] Agree
	- [ ] Neutral
	- [ ] Disagree
	- [ ] Strongly Disagree
	- [ ] Prefer not to say
54. How confident do you feel about using password managers?  
Mark only one oval.
	- [ ] Extremely confident
	- [ ] Somewhat confident
	- [ ] Neutral
	- [ ] Somewhat not confident
	- [ ] Extremely not confident
	- [ ] Prefer not to say

## 16. Continuing on Password Managers
55. Do you **prefer** to use password managers for saving passwords for **Online Banking** websites?  
Mark only one oval.
	- [ ] Yes
	- [ ] No
	- [ ] Prefer not to say
	- [ ] Maybe
56. Do you **prefer** to use password managers for saving passwords for **Social Media** websites?  
Mark only one oval.
	- [ ] Yes
	- [ ] No
	- [ ] Prefer not to say
	- [ ] Maybe
57. Do you **prefer** to use password managers for saving passwords for **e-commerce** (Amazon, Flipkart, etc.) websites?  
Mark only one oval.
	- [ ] Yes
	- [ ] No
	- [ ] Prefer not to say
	- [ ] Maybe
	
## 17. Let's see Password Managers a bit more!
58. Did the videos/tutorials influence your preference for using password managers over traditional methods?  
Mark only one oval.
	- [ ] Yes
	- [ ] No
	- [ ] Prefer not to say
59. After watching the videos, how easy do you think it is to set up and use password managers?  
Mark only one oval.
	- [ ] Very easy
	- [ ] Somewhat easy
	- [ ] Neutral
	- [ ] Somewhat difficult
	- [ ] Extremely difficult
	- [ ] Prefer not to say
	
## 18. Data-leaks on Password Managers
LastPass is a popular password manager service, which suffered a data 
leak, revealing a lot of information which was thought to be protected 
by the service such as websites in which a person has an account, their 
username and any URL parameters used by the website.

60. If you are made aware of a data leak / hack on your password manager, would you still continue using it?  
Mark only one oval.
	- [ ] Yes
	- [ ] No
	- [ ] Prefer not to say
	- [ ] Maybe
	
## 19. Recovery on Password Managers
A password manager that lets you reset your master password with a link or OTP is not truly "zero knowledge". This means they can somehow access your passwords if needed. Any recovery option is also a potential way for hackers to get your passwords.

61. After reading the above information, would you prefer a manager with a recovery option or without it?  
Mark only one oval.
	- [ ] With recovery
	- [ ] Without recovery
	- [ ] Prefer not to say
	- [ ] Maybe
62. Some applications that support data sync/backup ask you to re-enter your master password from time to time, so that you remember it longer. How often would you prefer to be prompted for the same?  
(master password: password to login to the password manager)  
Mark only one oval.
	- [ ] Once a month
	- [ ] Quarterly
	- [ ] Bi-Annually
	- [ ] Annually
	- [ ] Never
	- [ ] Prefer not to say
63. How would you prefer to recover your passwords, in case you forgot your password manager’s master password?  
(master password: password to login to the password manager)  
Mark only one oval.
	- [ ] Reset Master Password with Link to registered email
	- [ ] Reset Master Password with Link + OTP to your phone
	- [ ] Recovery Code from when you first setup the password manager
	- [ ] Prefer not to say
	- [ ] Other: _______________________________

## 20. Overall 2FA and Password Managers
Understanding that various threats exist even when one is using these security services and being aware of the fact that it may not be foolproof. (Explaining hackers' motives and various incidents that occurred to hack into devices that had password managers and 2FA services subscribed.)

64. Have you ever come across news or incidents involving security breaches related to password managers or compromised 2FA systems?  
Mark only one oval.
	- [ ] Yes
	- [ ] No
	- [ ] Prefer not to say
65. How many incidents involving security breaches related to password managers or compromised 2FA systems have you come across in the past 6 months?  
Mark only one oval.
	- [ ] More than 10
	- [ ] 5-10
	- [ ] 1-4
	- [ ] 0
	- [ ] Prefer not to say
66. How confident are you that you'd notice if someone tried to trick you into giving up your password manager’s password or extra security code(2FA)?  
Mark only one oval.
	- [ ] Very confident
	- [ ] Confident
	- [ ] Neutral
	- [ ] Not so confident
	- [ ] Not confident at all
	- [ ] Prefer not to say
67. In the context of ongoing threats to cybersecurity, how often do you update your knowledge about new attack methods and strategies used by hackers to compromise password managers?  
Mark only one oval.
	- [ ] Often
	- [ ] Sometimes
	- [ ] Rarely
	- [ ] Never
	- [ ] Prefer not to say
68. Are there any specific aspects of password managers and 2FA that you found particularly challenging?   \____________________
69. In your opinion, how valuable are password managers and 2FA in today's digital landscape?  
Mark only one oval.
	- [ ] Extremely Valuable
	- [ ] Valuable
	- [ ] Neutral
	- [ ] Not very valuable
	- [ ] Not valuable at all
70. Given the possibility of new and evolving threats, how important do you consider staying updated on best practices and security measures for password managers?  
Mark only one oval.
	- [ ] Extremely important
	- [ ] Somewhat important
	- [ ] Neutral
	- [ ] Somewhat not important
	- [ ] Extremely not important
\end{markdown}
Referred tutorial videos: 
\begin{itemize}
    \item 2FA Introduction: \href{https://www.youtube.com/watch?v=AMOtB7XkTT4}{https://www.youtube.com/watch?v=AMOtB7XkTT4}
    \item 2FA Setup: \href{https://www.youtube.com/watch?v=kPopzdiGR-U}{https://www.youtube.com/watch?v=kPopzdiGR-U}
    \item Password Manager Introduction: \href{https://www.youtube.com/watch?v=2WHafjlRpFQ}{https://www.youtube.com/watch?v=2WHafjlRpFQ}
    \item Password Manager Setup: \href{https://www.youtube.com/watch?v=wGw8-gLXVhE}{https://www.youtube.com/watch?v=wGw8-gLXVhE}
\end{itemize}
